# Supplementary material for: Epitaxial strain control of hole-doping induced phases in a multiferroic Mott insulator Bi2FeCrO6
Source: arXiv:1807.01649 ancillary file (2018-07-11)
Supplement: Supplementary file 1 [file SupplementaryMaterial.pdf]

# Supplementary Material for "Epitaxial strain control of hole-doping induced phases in a multiferroic Mott insulator $Bi_2FeCrO_6$"

Paresh C. Rout[(1)] and Varadharajan Srinivasan[(1,2)]
*(1) Department of Physics, Indian Institute of Science Education and Research Bhopal, Bhopal 462 066, India and*
*(2) Department of Chemistry, Indian Institute of Science Education and Research Bhopal, Bhopal 462 066, India*

## DETAILS OF DFT CALCULATIONS

### Code and parameters

We have carried out DFT calculations, on Sr doped BFCO systems by using the Quantum-ESPRESSO Code [1] within the frame work of plane wave basis set. The generalized gradient approximation (GGA) exchange-correlation functional was used as per the Perdew-Burke-Ernzerhof (PBE) scheme [2, 3]. As these compound contains $3d$ transition metal (TM) ions (Fe,Cr), the correlation effect that arises from these TM electrons can not be completely accounted for by GGA alone. So the correlation effect that arises from Fe $3d$ and Cr $3d$ electrons were described by using GGA plus the on-site Hubbard $U$ (GGA+$U$) formulation [4–6]. We have used ultrasoft pseudopotentials for all the atoms in the structure. The kinetic energy cut-off and the charge density cut-off used for this calculations are 85 Ry and 800 Ry respectively. An $10 \times 10 \times 6$ Monkhorst-Pack grid of k point mesh were used for Brillouin zone integrations. However, for the density of states (DOS) and band structure calculations, the Monkhorst-Pack grid of k point mesh were increased to $14 \times 14 \times 10$. The electronic self-consistency cycles were converged down to $1.36 \times 10^{-11}$ eV and all the structures were relaxed until the Hellman-Feynman forces are less than 0.26 meV/Å. The Hubbard $U$ parameters were calculated using linear response theory of Ref. [5, 6]. The calculated $U$ values found to be of 4.25, 3.07 eV for Fe, Cr respectively, in the $Bi_2FeCrO_6$ system. The electronic contribution to the spontaneous polarization was calculated by using the Berry-phase method [7, 8].

For this calculation, we have constructed 20-atomic $\sqrt{2} \times \sqrt{2} \times 2$ tetragonal supercells like the original $Bi_2FeCrO_6$ structure (shown in Fig. 1 of main paper), starting from a simple cubic double-perovskite (DP) structure, to allow for appropriate magnetic ordering of ions along $(111)$ direction. The supercell chosen also allows us to incorporate the $P2_1/n$, as well as, $R3$ symmetries which is helpful in assessing the relative stability of the non-polar and polar phases. Apart from these two space group, we have also considered various other possible space groups such as $I4/m$, $Pbnm$, and $I4/mmm$ for the calculations, however, they are found to be higher in energy by 57 meV/f.u., 208 meV/f.u. and 781 meV/f.u., respectively as compared to the $R3$ structure at 0% strain. As we are interested in an epitaxial thin-films, by using the pseudo-cubic lattice parameter $a_{cub} = 3.93$Å [9](extracted from the bulk BFCO) as reference, we generated structures mimicking the epitaxially-strained films by varying the in-plane lattice parameters over a range of realistic substrate strains corresponding to (001) epitaxial growth.

After imposing the in-plane mechanical constraint, the out-of-plane lattice constant (c-lattice parameter) and all internal atomic positions are fully relaxed until the forces and the total energies reached the aforementioned thresholds. The $P2_1/n$ symmetry structure is characterized by an $a^-a^-c^+$ tilt pattern of the oxygen octahedra while that of ferroeletric $R3$ symmetry structure corresponds to an $a^-a^-a^-$ tilt pattern [10–12]. The $+(-)$ superscripts indicate in- (out-of)- phase rotations of adjacent octahedra along a given Cartesian direction. The structural stability of SBFCO depends on the ionic radii [13] of the constituent metal ions via the tolerance factor $t$ (Eq. 1) of the double-perovskites [14] ($A_2BB'O_6$):

$$\boxed{\mathbf{t} = \frac{\frac{\mathbf{r_A}}{\mathbf{2}} + \frac{\mathbf{r_{A'}}}{\mathbf{2}} + \mathbf{r_O}}{\sqrt{\mathbf{2}} \times (\frac{\mathbf{r_B}}{\mathbf{2}} + \frac{\mathbf{r_{B'}}}{\mathbf{2}} + \mathbf{r_O})}} \tag{1}$$

where $r_A$, $r_{A'}$, $r_B$, and $r_{B'}$ are the ionic radii of the respective ions and $r_O$ is the ionic radius of oxygen. The crystal structure of SBFCO was carefully chosen for our calculations since it has a tolerance factor of 0.96 (50% Sr) and 0.93 (25% Sr), indicating the perovskite structure is highly susceptible to $FeO_6$ and $CrO_6$ octahedral rotations about the principal symmetry axes.

## MAGNETIC AND CATION ORDERING STRUCTURES

We have taken three possible types of AFM ordered structures - A, C, G-types and FM ordered structures as shown in Fig.1(a). In each of these magnetic orders we incorporated the layered (D1) and the rock-salt ordered (D0) arrangements of Fe/Cr ions in the supercell, as shown in the Fig. 1(b). All the structures were fully relaxed and the final GGA+$U$ energies were plotted against epitaxial strain (see main text).

## STRUCTURAL OPTIMIZATION

Total energies in all the figures are plotted with respect to the lowest energy state among all i.e with respect to D0 ($R3$) FM state at +1% strain.

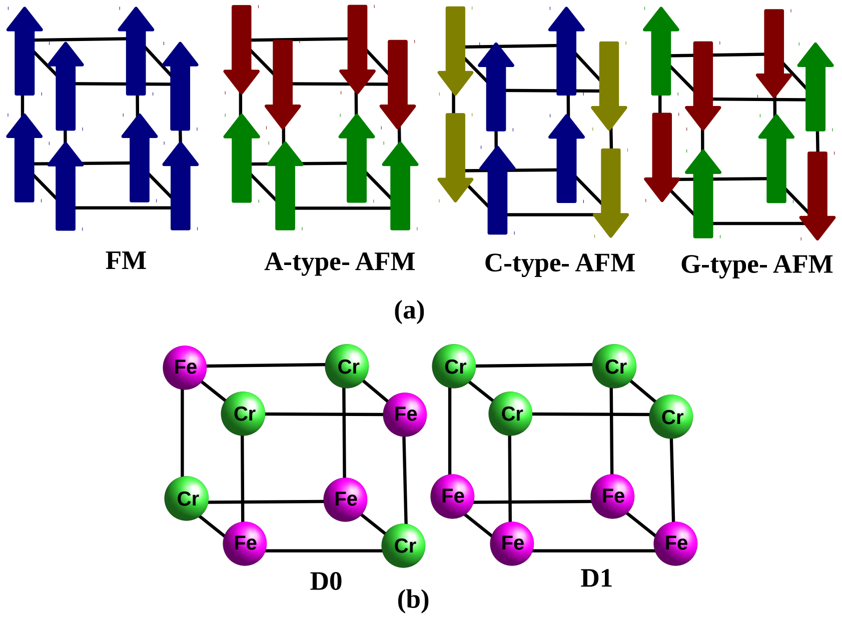


FIG. 1. Different types of cells considered in the calculations differing in : (a) magnetic ordering, where with up and down arrows representing up and down spins, respectively. FM refers to a ferromagnetic ordering where as A-, C- and G-types are different types of antiferromagnetic orderings and (b) Possible cation (Fe/Cr) ordering, which provides D0 and D1 structures

**Effect of epitaxial strain on $\mathbf{Bi_{2-x}Sr_xFeCr_6}$ ($x = 1$)**

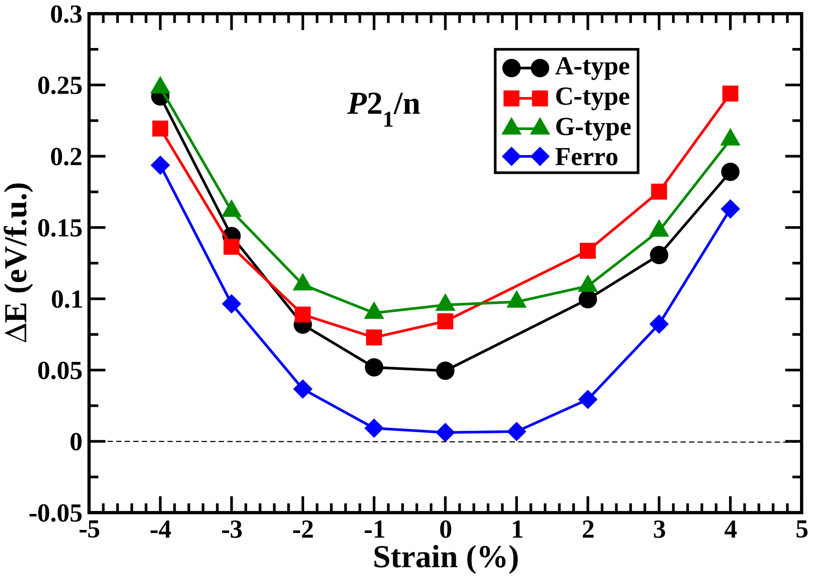


FIG. 2. Evolution of total energy of D0 $BiSrFeCrO_6$ in $P2_1/n$ symmetry. Total energy per formula unit of various magnetic ordered structure as a function of epitaxial strain. The blue line represents ferromagnetic (FM) state; black line, A-type AFM; red line, C-type AFM and the solid green line, G-type AFM. All the energies are positioned with respect to the lowest energy state ($R3$ FM state at 1% strain).

After following the structural optimization for D0 structure, we observed that the FM state emerged as the ground state under all epitaxial strains and the C-type AFM, denoted by solid red line, remain energetically higher at all strains. So, the C-type AFM ordering, which was the ground state and the main cause for low magnetic moment in pure $Bi_2FeCrO_6$ thin-films [15] is

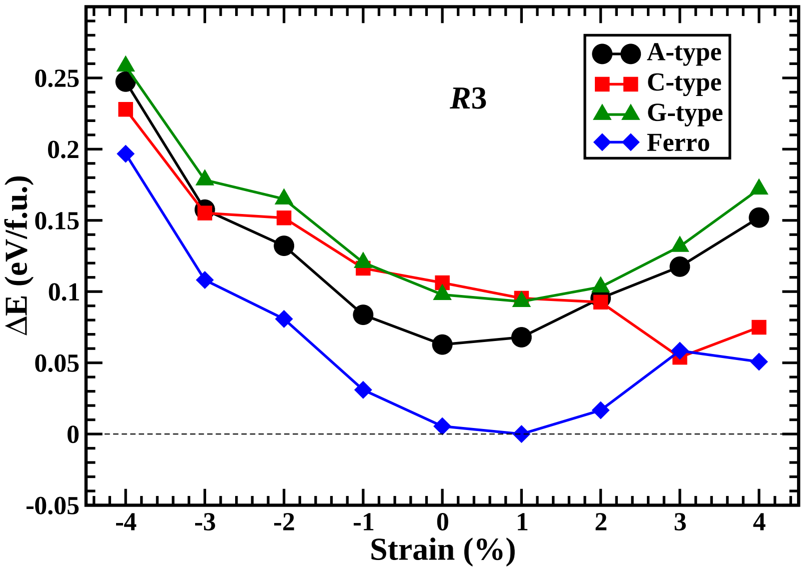


FIG. 3. Lowest energy structure of D0 $BiSrFeCrO_6$ in rhombohedral ($R3$) symmetry. Total energy per formula unit of various magnetic ordered structure as a function of epitaxial strain. The blue line represents ferromagnetic (FM) state; black line, A-type AFM; red line, C-type AFM and the solid green line, G-type AFM.

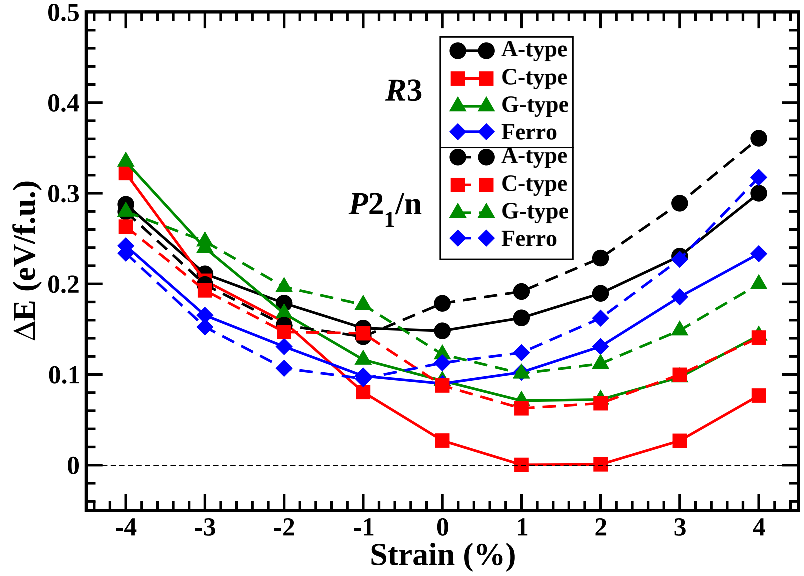


FIG. 4. Total energy per formula unit as a function of in-plane lattice parameters (epitaxial strain) of 50% Sr-doped D1 structure in both rhombohedral ($R3$) and monoclinic ($P2_1/n$) symmetry. The blue line represents ferromagnetic (FM) state; black line, A-type AFM; red line, C-type AFM and the solid green line, G-type AFM. Solid line and broken line depicts the $R3$ phase and $P2_1/n$ phase respectively. All the energies are calculated with respect to the lowest energy among all (C-type AFM of $R3$ phase at +1% strain).

destabilized by hole doping. Thus, the magnetic moments could in principle be improved in BFCO thin film through A-site Sr doping.

The same structural optimization were repeated for the Sr-doped cation disordered D1 structure of BFCO. This structure was shown to be the lowest in energy by Rout *et al.* [15]. The optimized energies are shown in Fig. 4. The solid coloured lines depict different magnetic orderings of $R3$ and the broken lines depict magnetic orderings of $P2_1/n$ phase. The results shown in Fig. 4 indicates that the C-type AFM of $R3$ phase is the lowest energy state under all tensile strain. At compressive strain higher than 1.2%, the antipolar (AP) $P2_1/n$ phase becomes more stable. Thus, there is a strain induced structural transition

in the D1 structure of SBFCO. We have also shown the $c/a$ axis ratio of stable structures with respect to epitaxial strain in Fig. 5. Although, there is no clear discontinuity in D0 $R3$ structure, a sharp discontinuity occurs in the $P2_1/n$ D0 structure at the vicinity of $c/a$ ~1.38. This is a clear indication of first-order phase transition at 0% strain in the D0 $P2_1/n$ phase.

In order to further characterize isosymmetric phase transitions, we have treated the octahedral rotation and tilts as order

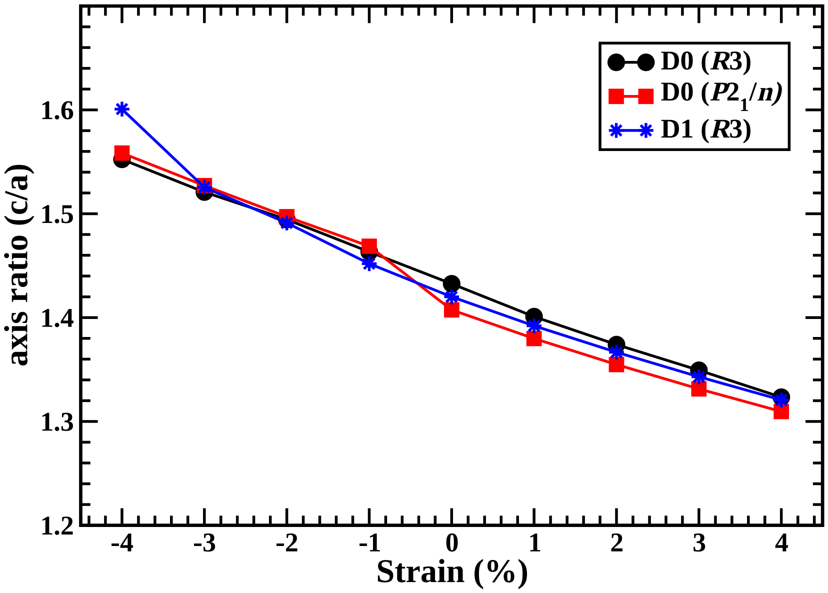


FIG. 5. Shows the strain *vs* $c$-axis plot for stable D0 and D1 cation ordered structure with various symmetry.

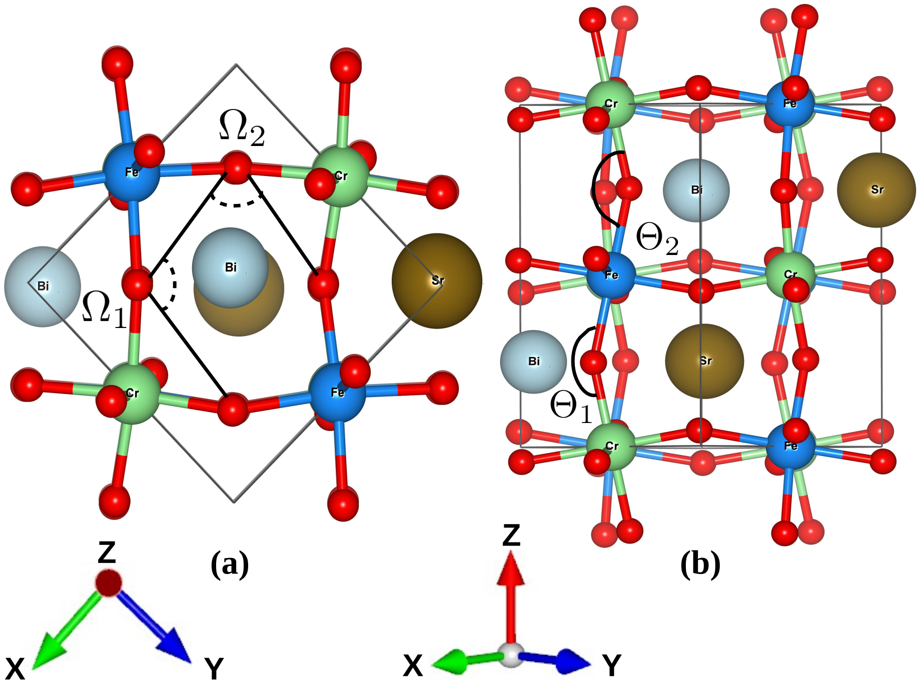


FIG. 6. The monoclinic $P2_1/n$ perovskite structure of SBFCO with tilting (rotation) of the octahedral cages.(a) The top view of the structure of SBFCO showing the distortion which we refer to as a rotation. The corner-connected oxygen octahedra rotate in opposite directions around the [001] direction.(b) The tilting of the SBFCO structure shown along [110] direction.The angles shown define degrees of tilting and rotation.

parameters. The tilt angle is defined as, $\alpha = (180 - \Theta)/2$ and the rotational angle is $\beta = (90 - \Omega)/2$, where $\Theta$ is the dihedral angle along Fe-O-Cr bond and $\Omega$ is an angle (see Fig. 6). There are two separate tilt angles ($\alpha_1$ and $\alpha_2$) and two rotational angles

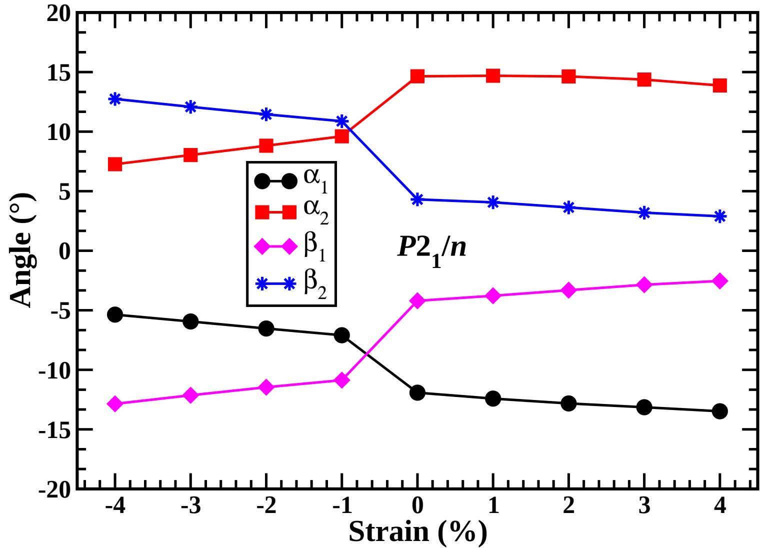


(a)

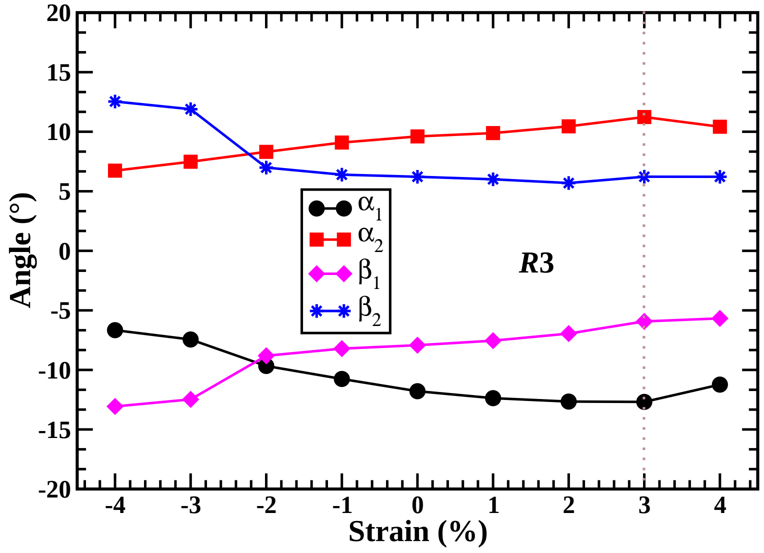


(b)

FIG. 7. Tilting and rotation angles of the oxygen octahedra as a function of strain. (a) Evolution in the $FeO_6$, $CrO_6$ octahedra rotation and tilt angles about [001] direction for $P2_1/n$ phase of D0 structure. (b) Evolution in the $FeO_6$, $CrO_6$ octahedra rotation and tilt angles about [001] direction for $R3$ phase of D0 structure. In the $P2_1/n$ phase both tilt and rotation sharply change at 0% strain leading to the IPT. Similarly, for $R3$ phase sudden change in angles is seen at -2% and +3% strain, pushing the system to an IPT.

($\beta_1$ and $\beta_2$) in the SBFCO unit cell, as it contains two separate TM (Fe, Cr) ions. Fig. 7 shows that for both the structural phases the oxygen octahedra rotation (OOR) around Cr atom ($\beta_1$) increases when the strain varies from the compressive to tensile, whereas the corresponding oxygen octahedra tilt (OOT) Fe-O-Cr ($\alpha_1$) shows the opposite behaviour. In both the $P2_1/n$ and $R3$ cases, under compressive strain, the tilting angles stay close to a value of 6°, while under tensile strain the tilting angles stay close to a value of 15°. Similarly, the rotation angles remain close to 14° under compressive strain for both the considered phases, while under tensile strain, the rotational angles varied differently and stay close to 4°, 5° for $P2_1/n$, $R3$ phases, respectively.

We decompose the structural distortion of $P2_1/n$ and $R3$ phases with respect to their ideal non-tilted [001] oriented double perovskite $P4/mmm$ structure by using the AMPLIMODES software [16]. From this calculation, we note that, the dependence

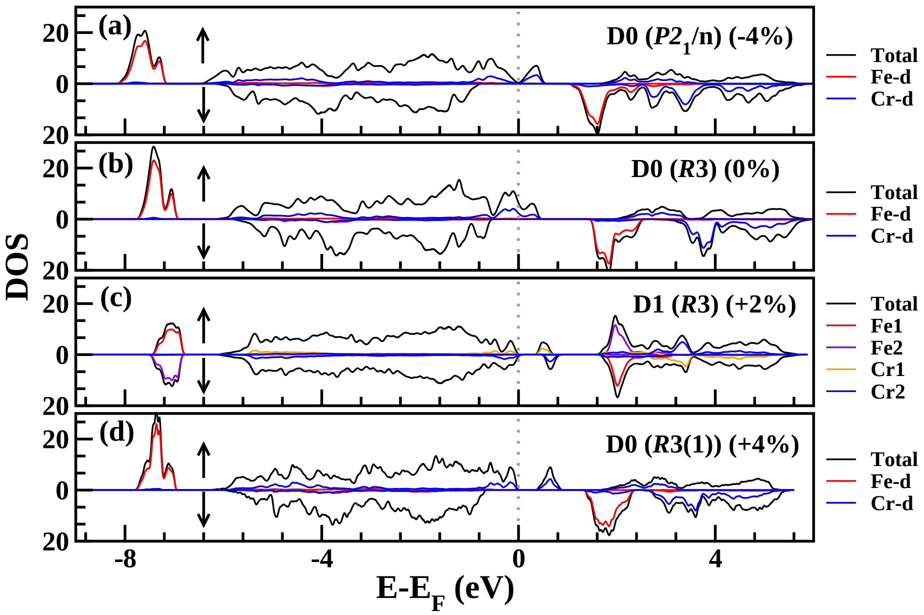


FIG. 8. Total and projected density of states (PDOS) of lower energy phases of Sr doped BFCO structure under epitaxial strain. The zero energy marks the position of Fermi energy ($E_f$) (a) PDOS plot for the antipolar ($P2_1/n$) phase -4% strain, (b) Atom-projected density of states for the polar $R3$ phase at 0% strain, (c) PDOS for the polar ($R3$) D1 structure at +2% strain and (d) show the PDOS for isosymmetric polar structure ($R3(1)$) at +4% strain.

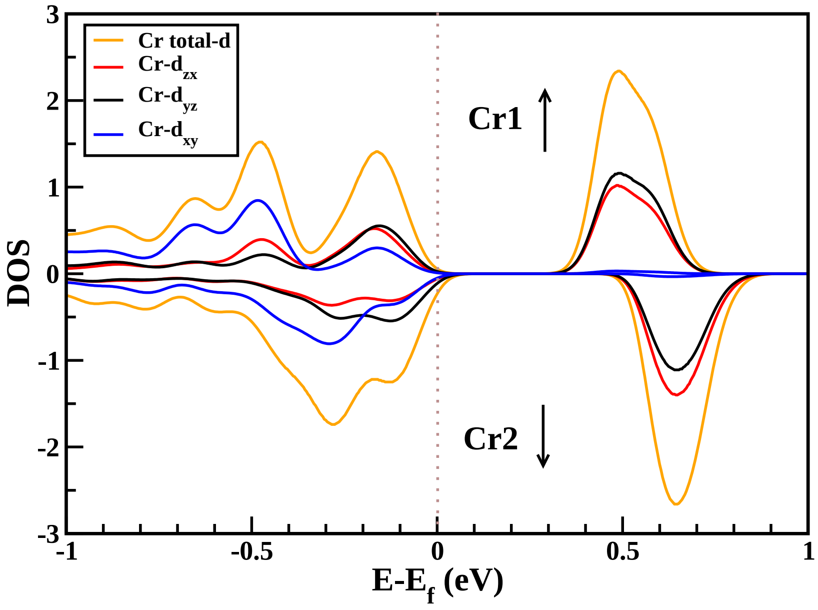


FIG. 9. Zoomed in view of total and projected density of states (PDOS) for the $d$-orbitals of polar ($R3$) D1 structure at +2% strain. The zero energy marks the position of Fermi energy ($E_f$). Hole states sit on the $d_{xz}/d_{yz}$ orbitals leading to ferro orbital ordering.

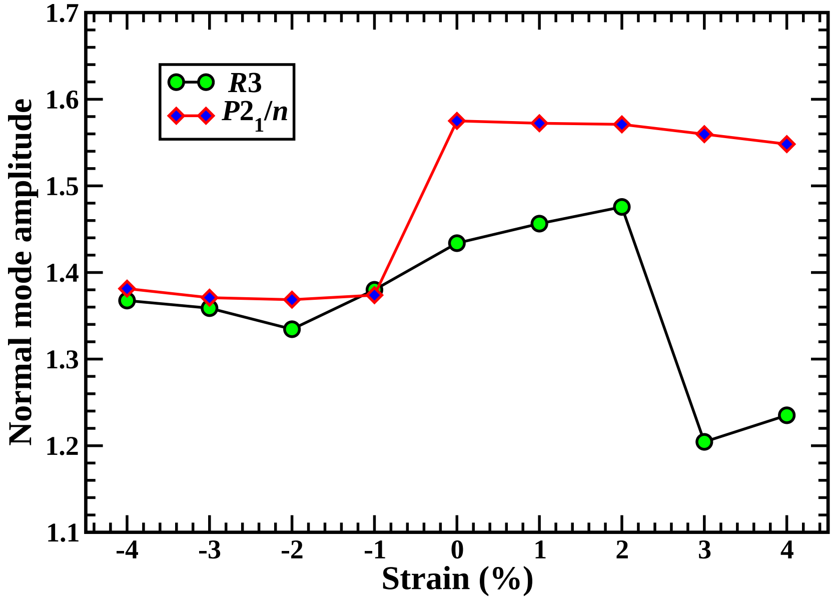


FIG. 10. Normalized displacement mode amplitudes ($\Gamma_1$) for $P2_1/n$ and $R3$ structures corresponding to oxygen octahedra rotation and oxygen octahedra tilt with respect to applied strain.

of rotation and tilt angles on in-plane epitaxial strain are qualitatively identical to those of the corresponding symmetry adapted modes (Compare both Fig.4 (main text) and Fig. 10). The Fig. 10 depicts the displacement (normal mode) amplitudes of

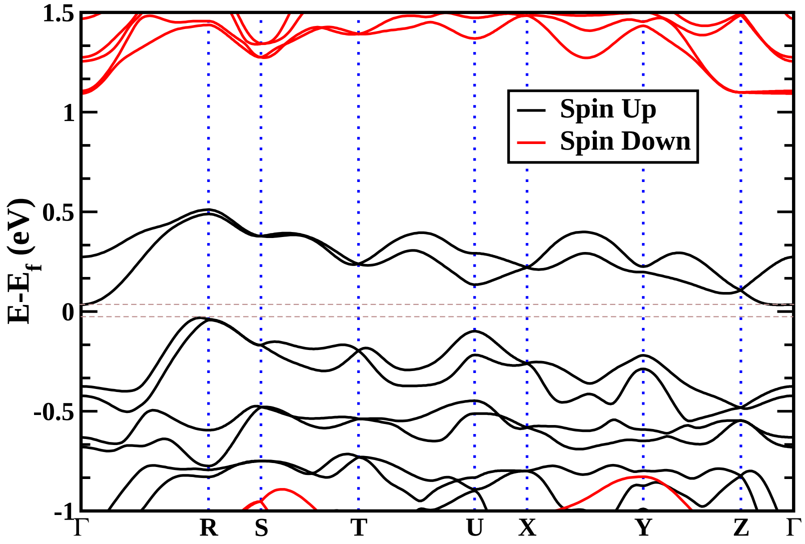


FIG. 11. Calculated band dispersion for the antipolar ($P2_1/n$) phase of SBFCO structure at -4% strain. The zero energy marks the position of Fermi energy ($E_F$). The black line stands for the spin up channel bands and the red line represents the spin down states. The valence and conduction band edges are indicated by dashed horizontal lines. The dotted, vertical lines in the plot mark the position of high-symmetric **k** points.

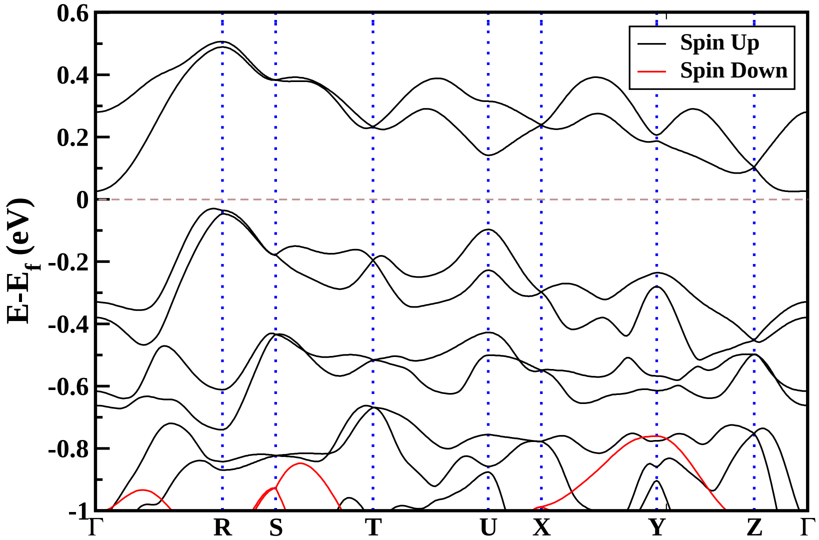


FIG. 12. Calculated band dispersion for the antipolar ($P2_1/n$) phase of SBFCO structure at -3% strain. The zero energy marks the position of Fermi energy (E$_F$). The black line stands for the spin up channel bands and the red line represents the spin down states.

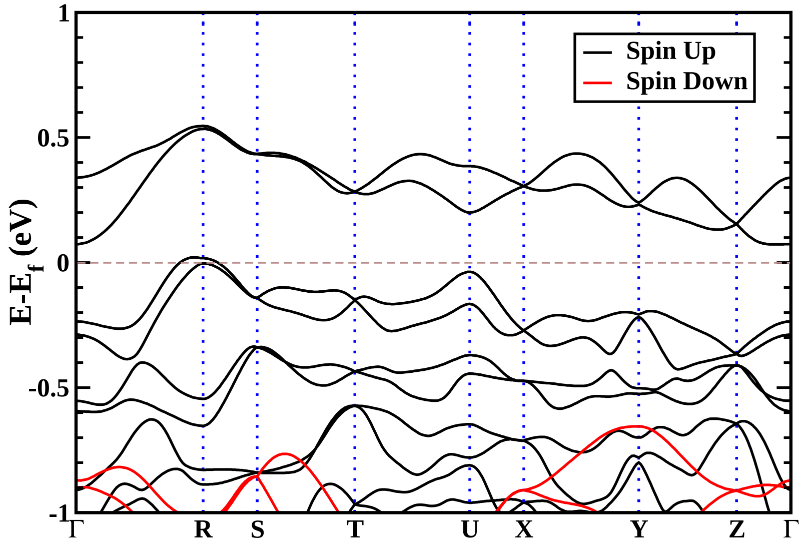


FIG. 13. Illustrates band dispersion for the antipolar ($P2_1/n$) phase of SBFCO structure at -2% strain. The zero energy marks the position of Fermi energy (E$_F$). The black line stands for the spin up channel bands and the red line represents the spin down states.

lowest energy structures across various epitaxial strain. The solid red line represents the Amplimodes for D0 monoclinic phase

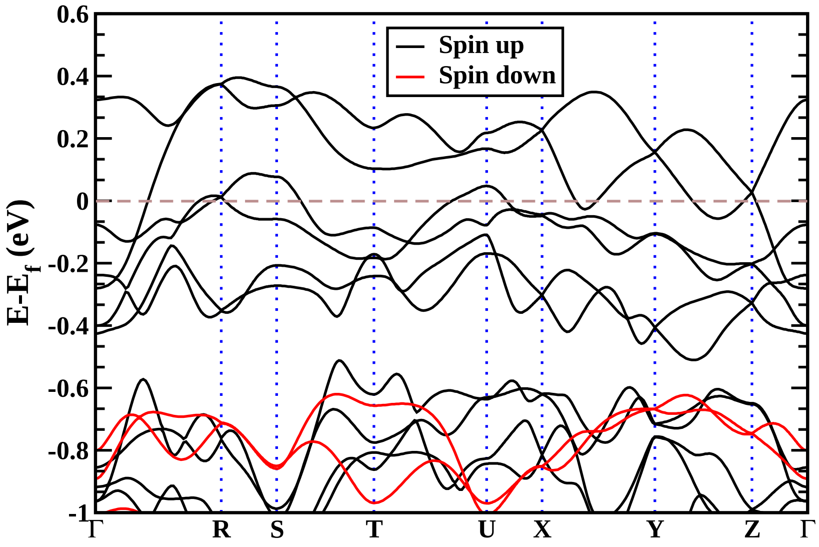


FIG. 14. Depicts the band dispersion for the polar ($R3$) phase of SBFCO structure at 0% strain. The dashed horizontal line at zero energy marks the position of Fermi energy ($E_F$). The black line stands for the spin up channel bands and the red line represents the spin down states. The dotted, vertical line in the plot marks the position of high-symmetric **k** points.

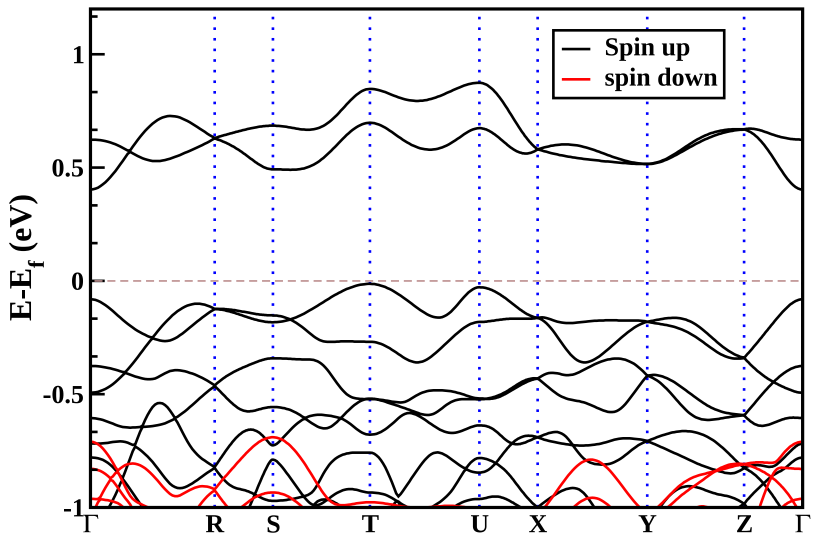


FIG. 15. Calculated band dispersion for the polar isosymmetric phase of SBFCO structure at +4% strain. The dashed horizontal green line at zero energy marks the position of Fermi energy ($E_F$). The black line stands for spin up channel bands and the red line represents the spin down states. The dotted, blue vertical line in the plot marks the position of high-symmetric **k** points of the Brillouin zone.

and solid black line stands for the polar D0 structure. However, for both the cases we have found one type of displacement mode amplitudes ($\Gamma_1$) for both the cases. As it can be seen from Fig. 10 that, the IPT of $R3$ structure can, in principle, be characterized by the evolution of $\Gamma_1$ modes as a function of in-plane strain, which again exhibit pronounced discontinuity at -2% and +2% strain. A very similar and sharp discontinuity also seen in $\Gamma_1$ modes at 0% strain of $P2_1/n$ structure, which again indicates the IPT at that strain point. The sharp discontinuity at different strain suggests that the isosymmetric phase transition is related to the sudden change in magnitude of displacement modes although being unstable for larger and smaller in-plane lattice parameters.

The Fig. 11 depicts the band dispersion of ferromagnetic $P2_1/n$ -phase of SBFCO structure at -4% strain in the energy range around the gap for the majority and minority spin channels. The band gap is indirect at this strain with the bottom of the conduction band located at the point Γ in the monoclinic Brillouin zone and the top of the valence band lying between Γ and R. We have also shown the band dispersion for the ferromagnetic $P2_1/n$ structure at -3% and -2% strain in Fig.12 and Fig.13, respectively. While the antipolar phase remains clearly an insulator at -3% strain, there is an indication of the valence band crossing the Fermi level around the R point at -2% strain. However, the density of states contributed by this crossing is too weak to deem the system metallic.

In contrast, at 0% strain there is a clear and robust half-metallic band structure as shown in Fig. 14. Only majority $up$ spin bands crosses Fermi level while the minority $down$ spin bands are far away from the Fermi level with a wide band gap, hence giving rise to an insulating solution in the minority channel.

### Effect of epitaxial strain on $Bi_{2-x}Sr_xFeCr_6$ ($x = 0.5$)

We have shown the energy $vs$ strain diagram (see Fig. 16 and 17) for different magnetic orderings of different structural phases at 25% Sr doping concentration. All the energies are placed with respect to their global minimum value. In Fig. 18, we have shown the correlation between charge difference of Cr atoms, total magnetic moment and compressive strain. We found that the charge disproportionation increases with increase in compressive strain. In order to strengthen our result, we have calculated the octahedral distortion factor (see Fig. 19) for the two Cr atoms and compared with the undoped parent compound. The octahedra distortion parameter (Δ) has been calculated by using the formula [17] as follows:

$$\Delta = \frac{1}{6}\sum_{n=1,6}[\frac{(\delta(n) - \langle\delta\rangle)}{\langle\delta\rangle}]^2, \quad (2)$$

where $\delta$ is a Cr-O bond length and $\langle\delta\rangle$ is the mean bond length in the $CrO_6$ octahedra. With increasing compressive strain the

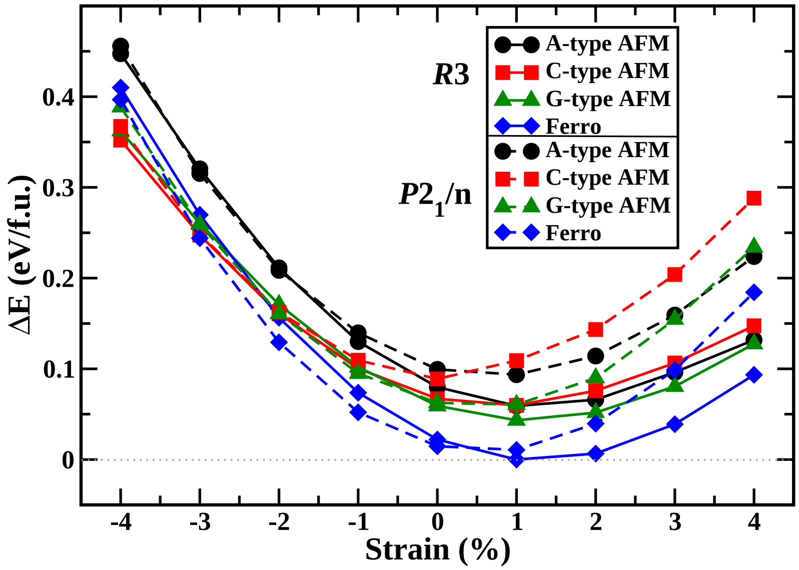


FIG. 16. Total energy per formula unit as a function of in-plane lattice parameters (epitaxial strain) of Sr-doped D0 structure in both rhombohedral ($R3$) and Monoclinic ($P2_1/n$) symmetry. The blue line represents ferromagnetic (FM) state; black line, A-type AFM; red line, C-type AFM and the solid green line, G-type AFM. Solid line and broken line depicts the $R3$ phase and $P2_1/n$ phase respectively. All the energies are calculated with respect to the lowest energy among all (FM phase D0 ($R3$) structure at +1% strain).

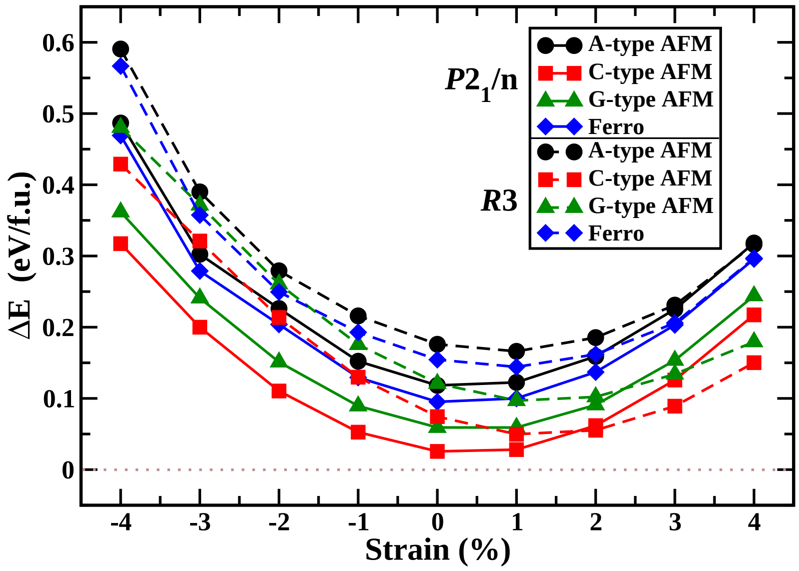


FIG. 17. Total energy per formula unit as a function of in-plane lattice parameters (epitaxial strain) of Sr-doped layered (D1) structure in both rhombohedral ($R3$) and Monoclinic ($P2_1/n$) symmetry. The blue line represents ferromagnetic (FM) state; black line, A-type AFM; red line, C-type AFM and the solid green line, G-type AFM. Solid line and broken line depicts the $P2_1/n$ phase and $R3$ phase respectively. All the energies are calculated with respect to the lowest energy among all (FM phase D0 ($R3$) structure at +1% strain).

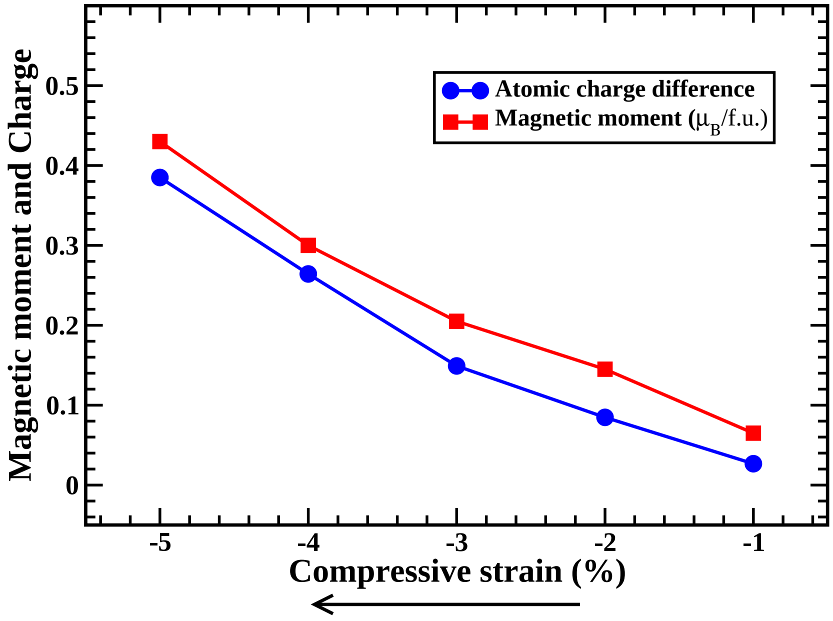


FIG. 18. Shows the atomic charge difference of two Cr atoms and magnetic moment per f.u. of C-type D1 structure at different compressive strain region.

octahedral distortions increases with different magnitude, however, in the undoped case the two octahedral distortions varies with same magnitude. This result clearly indicates the charge disproportionation in Cr-sites. Apart from this, we have also calculated the octahedral volume for the two Cr-sites and compared with the undoped parent compound BFCO (see Fig. 20). The octahedral volume has been calculated by using the formula $V = \frac{\sqrt{2}}{3}(\bar{a}^3)$, where $a$ is the edge of the octahedra. The octahedral volume decreases with increase in compressive strain. The octahedral volume remains constant for the two Cr-sites in the undoped case,

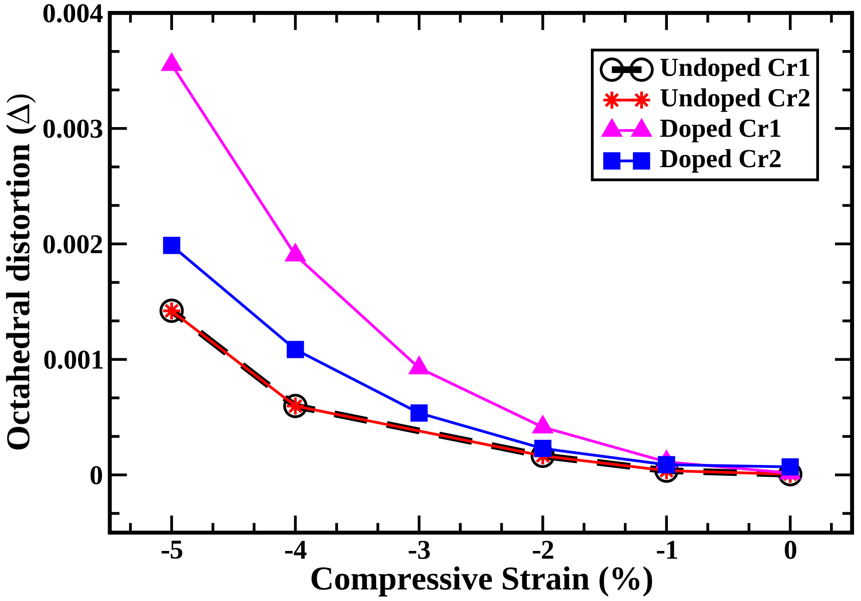


FIG. 19. Magnitude of octahedral distortion of the two Cr atoms in the C-type D1 structure at different compressive strain.

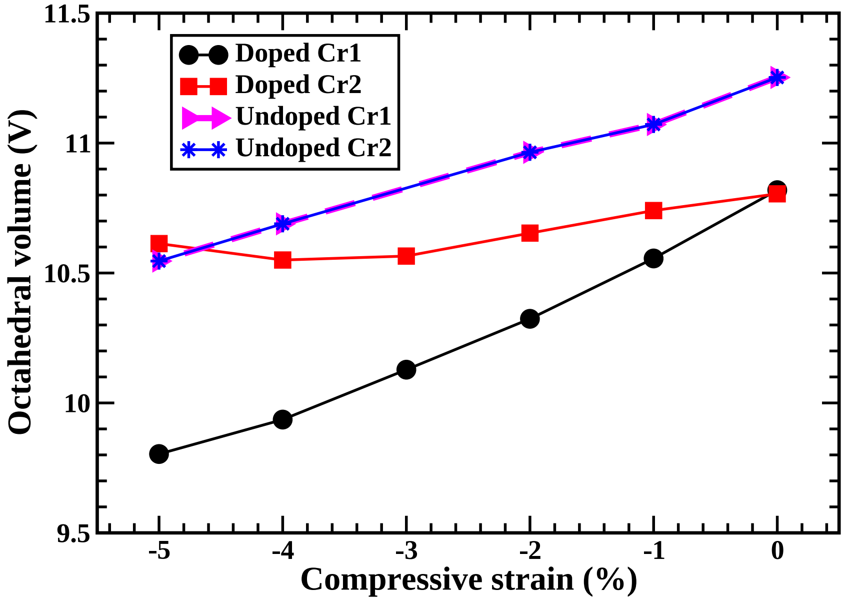


FIG. 20. Shows the variation of octahedral volume for two Cr atoms in C-type D1 structure at different compressive strain.

while in the doped structure the two octahedral volume are different, hence, confirming separate charges on the two Cr-sites at different strain region. As the charge disproportionation increases in the Cr-sites with increase in compressive strain, the oxygen octahedral volume difference also increases in the Cr-sites (see Fig. 20). The Fig. 18 depicts the correlation between charge

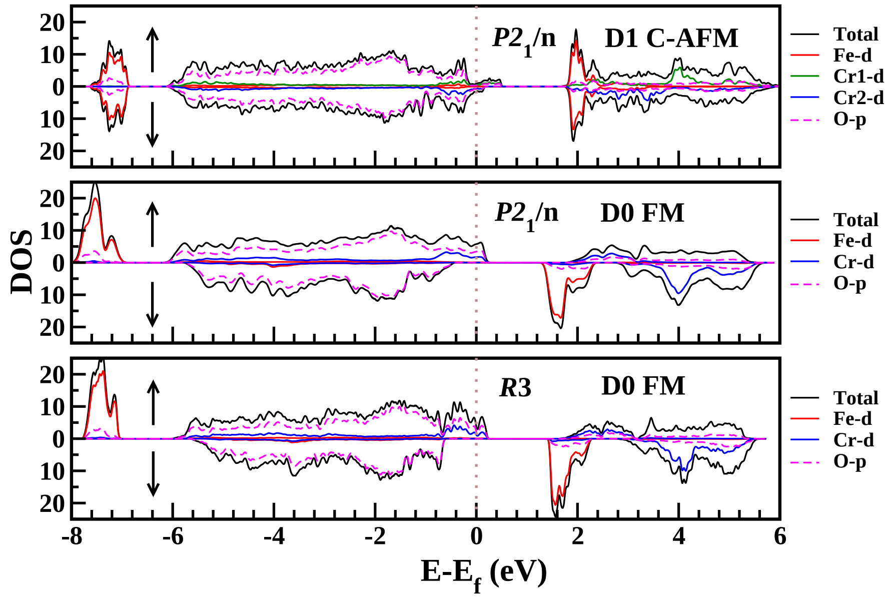


FIG. 21. Total and projected density of states (PDOS) of lower energy phases of Sr doped BFCO (25%) structure under epitaxial strain. The zero energy marks the position of Fermi energy ($E_F$) (a) PDOS plot for the antipolar ($P2_1/n$) phase of D1 structure at -4% strain, (b) Atom-projected density of states for the antipolar phase of D0 structure at 0% strain, and (c) represents the PDOS for the polar ($R3$) D0 structure at +4% strain.

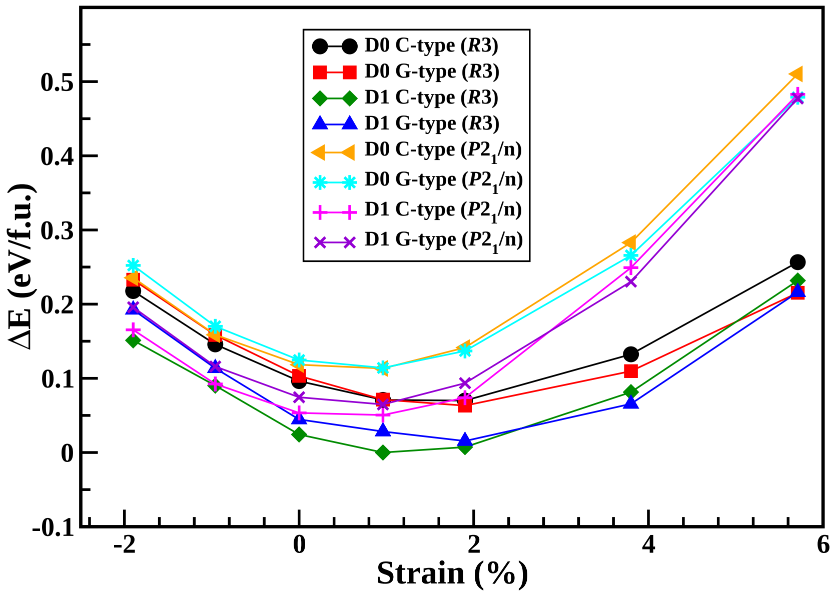


FIG. 22. Illustrates the energies of pure BFCO compound under various epitaxial strain.

difference with the residual magnetic moment of D1 C-type AFM. This clearly illustrates that the magnetic moment increases with increase in charge difference between the two Cr atom which clearly describes that the charge disproportionation increases with increase in compressive strain. However, the iron octahedra distortion remains unaffected under strain as the Sr atom unable to alter the oxidation state of Fe atoms.

Figure 22 illustrates the variation of total energies of the ground state structures (parent BFCO compound) with respect to

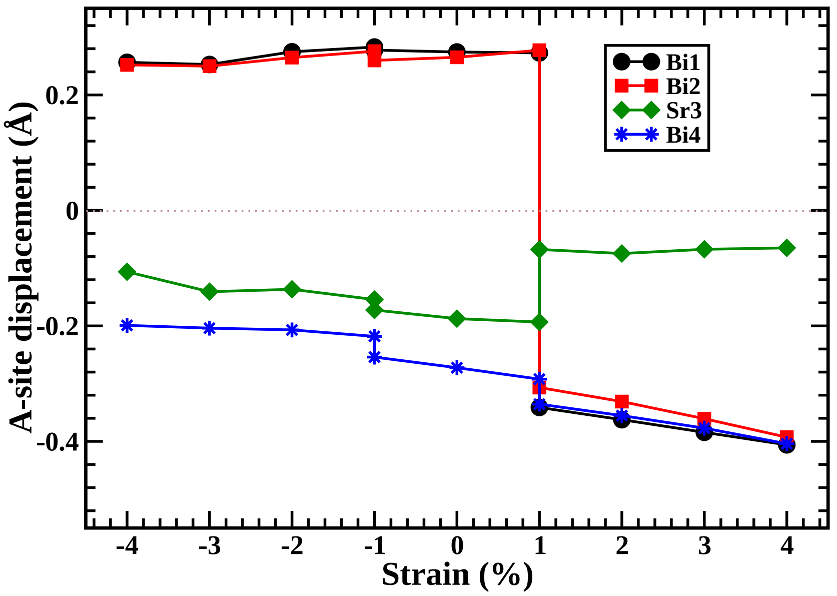


FIG. 23. Bi, Sr displacements ( in Å), along the pseudo-cubic [110] direction, from their respective positions in the ideal perovskite structure in 25% Sr-doped BFCO.

epitaxial strain. All energies are positioned with repect to their global minimum value. The layered D1-structure in C-type AFM configuration with $R3$ symmetry has been emerged as the the ground state in the coherent strain region (-2% to +2%).


[1] P. Giannozzi, S. Baroni, N. Bonini, M. Calandra, R. Car, C. Cavazzoni, D. Ceresoli, G. L. Chiarotti, M. Cococcioni, I. Dabo, A. D. Corso, S. de Gironcoli, S. Fabris, G. Fratesi, R. Gebauer, U. Gerstmann, C. Gougoussis, A. Kokalj, M. Lazzeri, L. Martin-Samos, N. Marzari, F. Mauri, R. Mazzarello, S. Paolini, A. Pasquarello, L. Paulatto, C. Sbraccia, S. Scandolo, G. Sclauzero, A. P. Seitsonen, A. Smogunov, P. Umari, and R. M. Wentzcovitch, Journal of Physics: Condensed Matter **21**, 395502 (2009).

[2] J. P. Perdew, K. Burke, and M. Ernzerhof, Phys. Rev. Lett. **77**, 3865 (1996).

[3] J. P. Perdew, K. Burke, and M. Ernzerhof, Phys. Rev. Lett. **78**, 1396 (1997).

[4] V. I. Anisimov, F. Aryasetiawan, and A. I. Liechtenstein, J. Phys. Condens. Matter **9**, 767 (1997).

[5] M. Cococcioni and S. de Gironcoli, Phys. Rev. B **71**, 035105 (2005).

[6] B. Himmetoglu, R. M. Wentzcovitch, and M. Cococcioni, Phys. Rev. B **84**, 115108 (2011).

[7] R. D. King-Smith and D. Vanderbilt, Phys. Rev. B **47** (1993).

[8] D. Vanderbilt and R. D. King-Smith, Phys. Rev. B **48** (1993).

[9] R. Nechache, C. Harnagea, A. Ruediger, F. Rosei, and A. Pignolet, FUNCT MATER LETT. **3**, 83 (2010).

[10] A. Glazer, Acta Crystallographica Section A: Crystal Physics, Diffraction, Theoretical and General Crystallography **31**, 756 (1975).

[11] A. Glazer, Acta Crystallographica Section B: Structural Crystallography and Crystal Chemistry **28**, 3384 (1972).

[12] P. M. Woodward, Acta Crystallographica Section B: Structural Science **53**, 32 (1997).

[13] R. D. Shannon, Acta crystallographica section A: crystal physics, diffraction, theoretical and general crystallography **32**, 751 (1976).

[14] H. P. S. Corrêa, I. P. Cavalcante, D. O. Souza, E. Z. Santos, M. T. D. Orlando, H. Belich, F. J. Silva, E. F. Medeiro, J. M. Pires, J. L. Passamai, L. G. Martinez, and J. L. Rossi, Cerâmica **56**, 193 (2010).

[15] P. C. Rout, A. Putatunda, and V. Srinivasan, Phys. Rev. B **93**, 104415 (2016).

[16] J. M. Perez-Mato, D. Orobengoa, and M. I. Aroyo, Acta Crystallographica Section A **66**, 558 (2010).

[17] J. M. Rondinelli and S. Coh, Phys. Rev. Lett. **106**, 235502 (2011).
